# Supplementary material for: Lumen: A Machine Learning Framework to Expose Influence Cues in Text
Source: arXiv:2107.10655 source file (2021-07-12)
Supplement: Supplementary file 1 [file _appendix_a.tex]

\appendices

\section{Supplementary material}\label{sec_appendix}

%-------------------------------------------------------------------------------
%\section{Appendix}

%-------------------------------------------------------------------------------

%\begin{figure}[!htb]
%	\centering
%	\includegraphics[width=.8\textwidth]{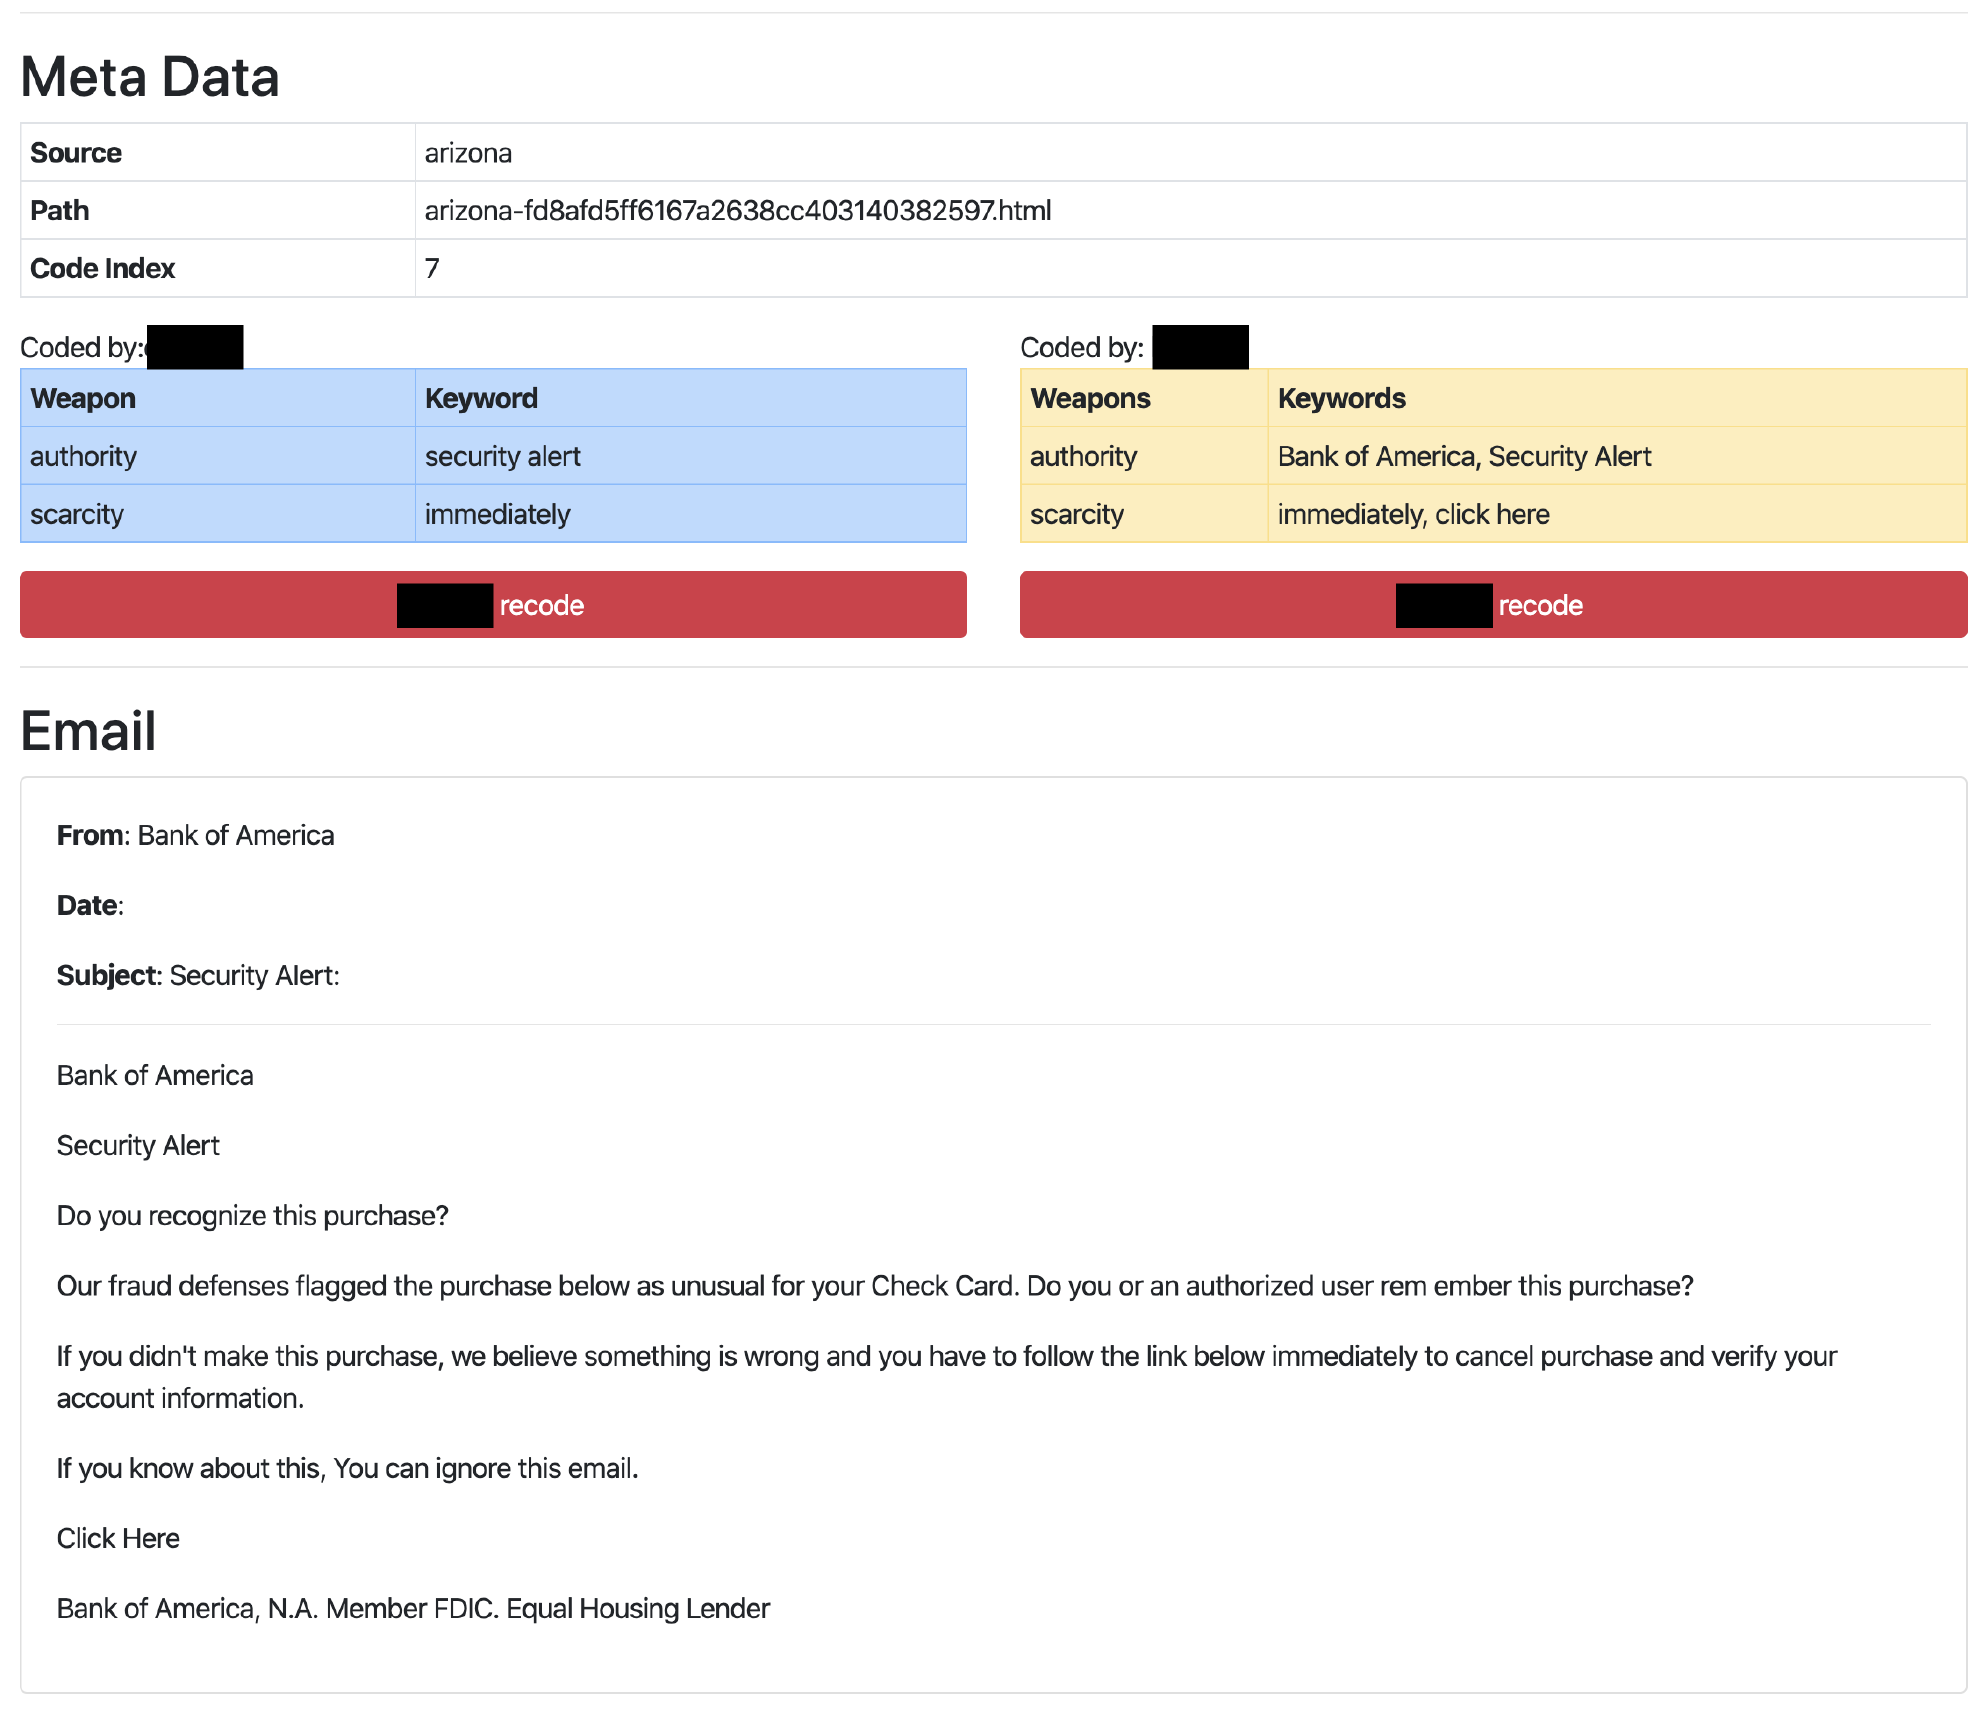}
%	\caption{\textbf{Screenshot of email browser.} Allowed for coders to address inconsistencies in coding. Here, both coders agreed that the email contained ``scarcity'' and ``authority''.}
%	\label{app_fig_Screenshot_of_email_browser}
%\end{figure}

\begin{figure*}[h]
	\centering
	\includegraphics[width=.6\textwidth]{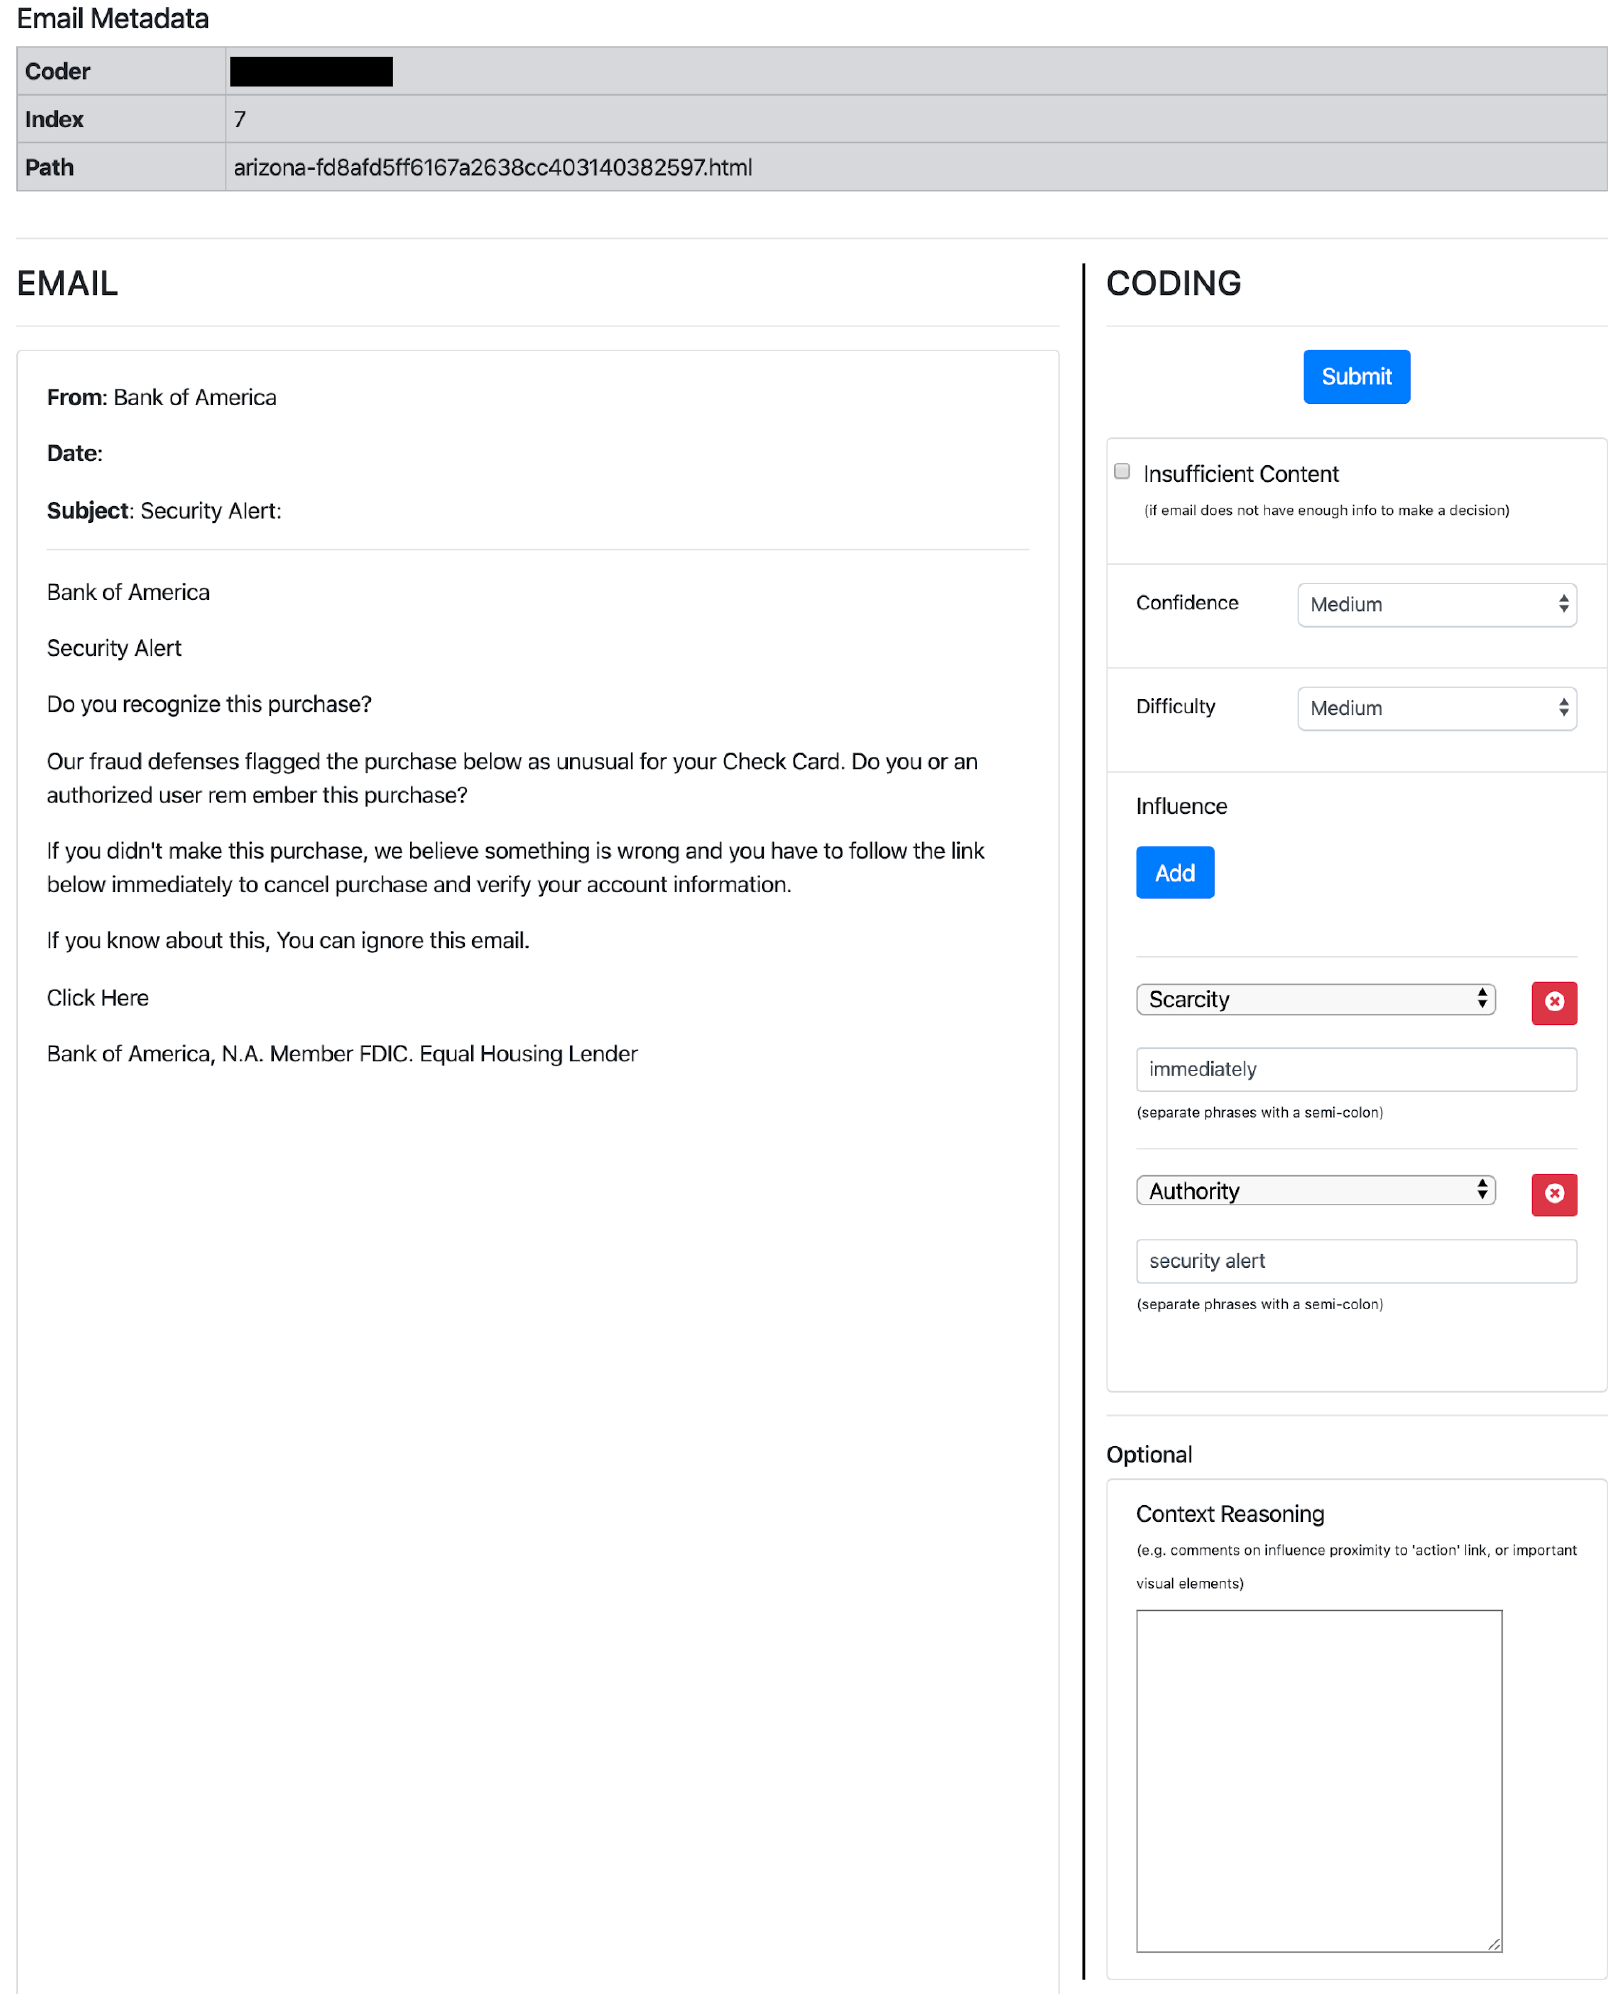}
	\caption{Screenshot of coding an email.}
	\label{app_fig_Screenshot_of_coding_an_email}
\end{figure*}

\begin{table*}[h!]
	\centering
	\caption{Distribution of emails found and coded as of this writing}
	\begin{tabular}{c|c|c}
		\hline
		Source  &   Number of Emails Found  &   Emails Coded    \\ \hline
		Arizona &   534 &   251 \\ \hline
		FTC &   57  &   8   \\ \hline
		Lehigh  &   81  &   6   \\ \hline
		University of Michigan  &   553 &   65  \\ \hline
		Miller Smiles   &   7,003   &   704 \\ \hline
		University of Minnesota &   8   &   8   \\ \hline
		Monkey.org  &   6,500   &   496 \\ \hline
		University of Pennsylvania  &   232 &   25  \\ \hline
		University of Pittsburgh    &   107 &   10  \\ \hline
		SPAM emails &   266 &   266 \\ \hline
		UCLA    &   158 &   19  \\ \hline
		University of Florida   &   69  &   6   \\ \hline
		Untroubled  &   69  &   69  \\ \hline
	\end{tabular}
	\label{app_table_email_found_coded}
\end{table*}

\begin{table*}[!htb]
	\centering
	\caption{Coding Manual: Definitions for persuasion and framing}
	\begin{tabular}{p{2cm}|p{7cm}|p{7cm}}
		\hline
Principle	&	Definition/how it influences people	&	Example(s)	\\ \hline
Scarcity	&	According to the principle of scarcity, opportunities seem more valuable when their availability is limited. When under time pressure to make an important choices, people tend to use a different decision strategy, and hustlers steer us toward one involving less reasoning.	&	Rare, shortage, limited supply, unique, limited offer, free, exclusive, now, today, don't delay, asap, immediately.
	\\ \hline
Authority	&	The principle of authority states that humans tend to comply with requests made by (perceived) figures of authority.	&	Police, parking authority, IT Department, HR Department, loan office, any government body (e.g., IRS), doctor, professor, Amazon, Twitter.	\\ \hline
Commitment	&	The commitment principle proposes that once humans have taken a stand, they will feel pressured to behave in line with their commitment.	&	1. I care about the environment and disaster relief...''; 2. All patriots who love America...; 3. Sign this petition; 4. Consider Bob, a dog lover who feels devastated when he learns about cases of animal abuse and is vocal on Facebook about this issue. An adversary can target Bob by sending him an email about a petition to end animal cruelty in makeup testing.	\\ \hline
Liking 	&	The liking principle assumes that humans tend to comply with requests from people they like or with whom they share similarities.	&	1. Consider Bob, an older adult active in his church. Bob will feel more at ease accepting a request coming from Dan, 68, member of the same church, than a request coming from Alice, 19, student at a local University; 2. It was a pleasure speaking with you. 3. References to being the same age, gender, group, etc.	\\ \hline
Reciprocation	&	The reciprocation principle is based on the notion that humans tend to repay, in kind, what another person has provided them.	&	Free samples (target must have a net gain before feeling need to return favor).	\\ \hline
Social Proof	&	The principle of social proof relies on the idea that people tend to mimic what the majority of others do or seem to be doing. 	&	1. Everyone is doing it; 2. [X] out of 10 [doctors, lawyers] recommend; 3. [X] in your [school, neighborhood] [applied/enrolled/used]; 4. [x] satisfied customers; 5. Advertising a malicious link that shows 2 million people have already clicked the link (e.g., YouTube video with 2 million views); 6. What every entrepreneur must know!	\\ \hline
Gain	&	People are likely to act in ways that benefit them in some way. A reward will increase the probability of a behavior.	&	1. Make \$500; 2. Lose 10 pounds.	\\ \hline
Loss	&	People are likely to act in ways that reduce loss/harm to them. Avoiding loss will increase the probability of a behavior.	&	1. Your email will be suspended; 2. You won't receive your paycheck; 3. Your house will be foreclosed.	\\ \hline
	\end{tabular}
	\label{app_table_code_manual}
\end{table*}
