# Supplementary material for: Lumen: A Machine Learning Framework to Expose Influence Cues in Text
Source: arXiv:2107.10655 source file (2021-07-12)
Supplement: Supplementary file 2 [file appendix_a.pdf]

# Appendices

Email Metadata

|       |                                               |
|-------|-----------------------------------------------|
| Coder |                                               |
| Index | 7                                             |
| Path  | arizona-fd8afd5ff6167a2638cc403140382597.html |

EMAIL

**From:** Bank of America

**Date:**

**Subject:** Security Alert:

Bank of America

Security Alert

Do you recognize this purchase?

Our fraud defenses flagged the purchase below as unusual for your Check Card. Do you or an authorized user remember this purchase?

If you didn't make this purchase, we believe something is wrong and you have to follow the link below immediately to cancel purchase and verify your account information.

If you know about this, You can ignore this email.

Click Here

Bank of America, N.A. Member FDIC. Equal Housing Lender

CODING

Submit

☐ Insufficient Content  
(if email does not have enough info to make a decision)

Confidence 

Medium

Difficulty 

Medium

Influence

Add

Scarcity

immediately

(separate phrases with a semi-colon)

Authority

security alert

(separate phrases with a semi-colon)

Optional

Context Reasoning  
(e.g. comments on influence proximity to "action" link, or important visual elements)

Figure A1: Screenshot of coding an email.

Table A1: Distribution of emails found and coded as of this writing

| Source                     | Number of Emails Found | Emails Coded |
|----------------------------|------------------------|--------------|
| Arizona                    | 534                    | 251          |
| FTC                        | 57                     | 8            |
| Lehigh                     | 81                     | 6            |
| University of Michigan     | 553                    | 65           |
| Miller Smiles              | 7,003                  | 704          |
| University of Minnesota    | 8                      | 8            |
| Monkey.org                 | 6,500                  | 496          |
| University of Pennsylvania | 232                    | 25           |
| University of Pittsburgh   | 107                    | 10           |
| SPAM emails                | 266                    | 266          |
| UCLA                       | 158                    | 19           |
| University of Florida      | 69                     | 6            |
| Untroubled                 | 69                     | 69           |

Table A2: Coding Manual: Definitions for persuasion and framing

| Principle     | Definition/how it influences people                                                                                                                                                                                                                                              | Example(s)                                                                                                                                                                                                                                                                                                                                                                 |
|---------------|----------------------------------------------------------------------------------------------------------------------------------------------------------------------------------------------------------------------------------------------------------------------------------|----------------------------------------------------------------------------------------------------------------------------------------------------------------------------------------------------------------------------------------------------------------------------------------------------------------------------------------------------------------------------|
| Scarcity      | According to the principle of scarcity, opportunities seem more valuable when their availability is limited. When under time pressure to make an important choices, people tend to use a different decision strategy, and hustlers steer us toward one involving less reasoning. | Rare, shortage, limited supply, unique, limited offer, free, exclusive, now, today, don't delay, asap, immediately.                                                                                                                                                                                                                                                        |
| Authority     | The principle of authority states that humans tend to comply with requests made by (perceived) figures of authority.                                                                                                                                                             | Police, parking authority, IT Department, HR Department, loan office, any government body (e.g., IRS), doctor, professor, Amazon, Twitter.                                                                                                                                                                                                                                 |
| Commitment    | The commitment principle proposes that once humans have taken a stand, they will feel pressured to behave in line with their commitment.                                                                                                                                         | 1. I care about the environment and disaster relief..."; 2. All patriots who love America...; 3. Sign this petition; 4. Consider Bob, a dog lover who feels devastated when he learns about cases of animal abuse and is vocal on Facebook about this issue. An adversary can target Bob by sending him an email about a petition to end animal cruelty in makeup testing. |
| Liking        | The liking principle assumes that humans tend to comply with requests from people they like or with whom they share similarities.                                                                                                                                                | 1. Consider Bob, an older adult active in his church. Bob will feel more at ease accepting a request coming from Dan, 68, member of the same church, than a request coming from Alice, 19, student at a local University; 2. It was a pleasure speaking with you. 3. References to being the same age, gender, group, etc.                                                 |
| Reciprocation | The reciprocation principle is based on the notion that humans tend to repay, in kind, what another person has provided them.                                                                                                                                                    | Free samples (target must have a net gain before feeling need to return favor).                                                                                                                                                                                                                                                                                            |
| Social Proof  | The principle of social proof relies on the idea that people tend to mimic what the majority of others do or seem to be doing.                                                                                                                                                   | 1. Everyone is doing it; 2. [X] out of 10 [doctors, lawyers] recommend; 3. [X] in your [school, neighborhood] [applied/enrolled/used]; 4. [x] satisfied customers; 5. Advertising a malicious link that shows 2 million people have already clicked the link (e.g., YouTube video with 2 million views); 6. What every entrepreneur must know!                             |
| Gain          | People are likely to act in ways that benefit them in some way. A reward will increase the probability of a behavior.                                                                                                                                                            | 1. Make \$500; 2. Lose 10 pounds.                                                                                                                                                                                                                                                                                                                                          |
| Loss          | People are likely to act in ways that reduce loss/harm to them. Avoiding loss will increase the probability of a behavior.                                                                                                                                                       | 1. Your email will be suspended; 2. You won't receive your paycheck; 3. Your house will be foreclosed.                                                                                                                                                                                                                                                                     |
